# Supplementary material for: Experimental quantum decoherence control by dark states of the environment
Source: arXiv:2005.07169 source file (2020-05-14)
Supplement: Supplementary file 1 [file Supplement.pdf]

# Experimental quantum decoherence control by dark states of the environment

Robert Stárek, Michal Mičuda, Ivo Straka, Martina Nováková,
Miloslav Dušek, Miroslav Ježek, Jaromír Fiurášek, and Radim Filip
*Department of Optics, Palacký University, 17. listopadu 1192/12, 771 46 Olomouc, Czech Republic*

## SUPPLEMENTARY MATERIALS

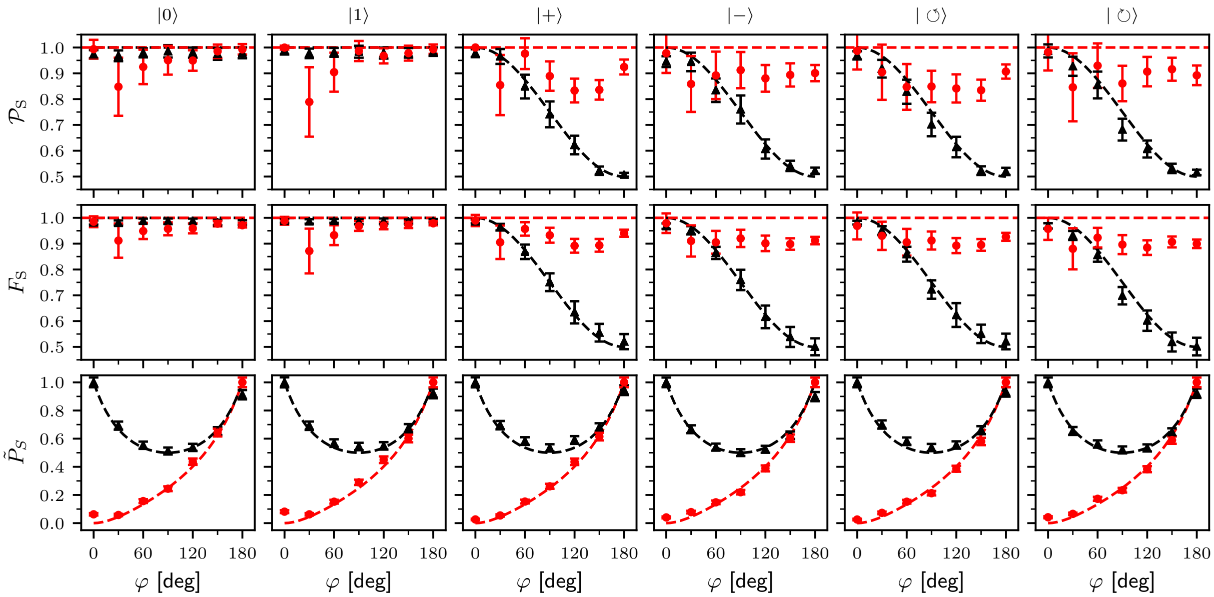


FIG. S1. The figure shows results of similar measurements as in Fig. 2. However, the environmental qubit is initially prepared in a pure state $|+\rangle_{\mathrm{E}}$ instead of the maximally mixed state.

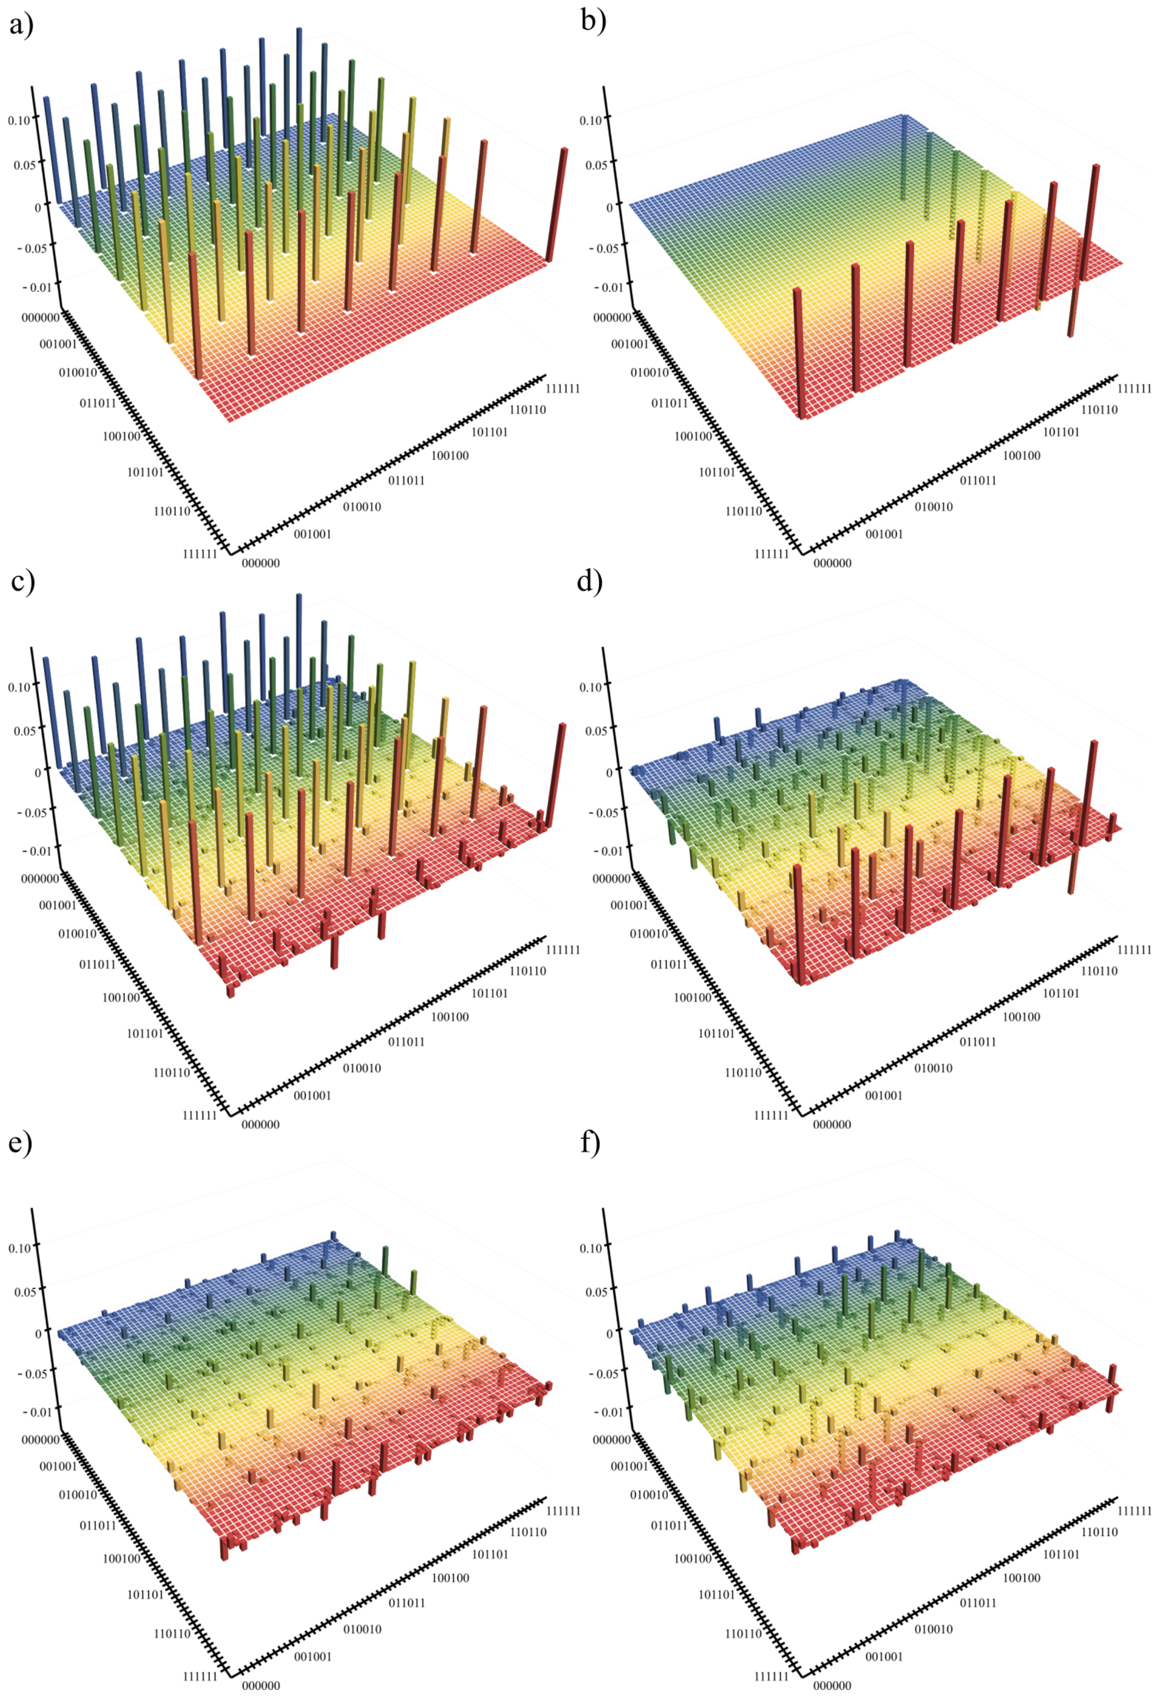


FIG. S2. Quantum process of the controlled-controlled-phase gate for $\varphi = \pi/2$. Shown are the real (a,c) and imaginary (b,d) parts of the quantum process matrix $\chi$. Experimental results plotted in panels (c,d) can be compared with the theoretical process matrix of the ideal theoretical unitary gate in panels (a,b). Real and imaginary parts of differences between experimental and theoretical matrices are plotted in panels (e) and (f), respectively.
